# Supplementary material for: Interval Spacing
Source: arXiv:2601.22116 source file (2026-08-21)
Supplement: Supplementary file 1 [file interval_spacing_supplement.tex]

% We keep this a separate document rather than making appendices to the
% main paper, so we don't have to worry about the page margins, which must
% be wide to handle the equations.

\documentclass[fleqn]{article}

\usepackage{amsmath}
\usepackage{graphicx}
\usepackage{authblk}

% Extend margins - this isn't for publication.
\addtolength{\oddsidemargin}{-1.25in}
\addtolength{\evensidemargin}{-1.25in}
\addtolength{\topmargin}{-1in}
\addtolength{\textwidth}{2.5in}
\addtolength{\textheight}{2in}
\fontsize{9}{12}

\begin{document}

\title{Supplement to {\em Interval Spacing}}
\author{Greg Kreider}
\affil{\small gkreider@primachvis.com}
\affil{\small Primordial Machine Vision Systems, Inc.}
\date{}

\maketitle

%%%%
\section*{Derivation of Equations}

We use
\begin{equation*}
S_{1} = \frac{n!}{(i-w-1)! (w-1)! (n-i)!}
\end{equation*}
throughout to denote the scaling factor before the density function, as in
the main text.

The density of the interval spacing is
\begin{align} \label{eq:fdiw.gen}
f_{D_{i,w}}(y) & =
\begin{aligned}[t]
  S_{1} \int_{-\infty}^{\infty} &
  \left\{ F_{x}(x) \right\}^{i-w-1} \left\{ F_{x}(x+y) - F_{x}(x) \right\}^{w-1}
  \left\{ 1 - F_{x}(x+y) \right\}^{n-i} \\
  & \times f_{x}(x) f_{x}(x+y) dx
\end{aligned} \\
\end{align}
The expected value and variance follow from the first and second moments.
\begin{align} \label{eq:ediw.gen}
E\Bigl\{ D_{i,w} \Bigr\}
 & = \int_{0}^{\infty} y ~ f_{D_{i,w}}(y) ~ dy
     \displaybreak[0] \\
\label{eq:vdiw.gen}
V\Bigl\{ D_{i,w} \Bigr\}
 & = E\Bigl\{ D_{i,w}^2 \Bigr\} - E\Bigl\{ D_{i,w} \Bigr\}^2 
   = \int_{0}^{\infty} y^{2} ~ f_{D_{i,w}}(y) ~ dy - E\Bigl\{ D_{i,w} \Bigr\}^2
\end{align}

%%%
\subsection*{Interval Spacing for Uniform Variates}

\renewcommand{\theequation}{U.\arabic{equation}}
\setcounter{equation}{0}

The variate's density and distribution functions are
\begin{align} \label{appeq:pcdf.unif}
f_{unif}(x) & = \frac{1}{b-a} \\
F_{unif}(x) & = \frac{x-a}{b-a}
\end{align}
for $ a \leq x \leq b $, with $ f(x) $ zero outside this range and $ F(x) $
zero below and one above.

\subsubsection*{Density Function}

\begin{align*}
f_{D_{i,w,unif}}(y)
 & = S_{1}
    \int_{-\infty}^{\infty}
      \left\{ \frac{x-a}{b-a} \right\}^{i-w-1}
      \left\{ \frac{x+y-a}{b-a} - \frac{x-a}{b-a} \right\}^{w-1}
      \left\{ 1 - \frac{x+y-a}{b-a} \right\}^{n-i} f(x) ~ f(x+y) ~ dx \\
 & = S_{1}
    \int_{-\infty}^{\infty}
      \left\{ \frac{x-a}{b-a} \right\}^{i-w-1}
      \left\{ \frac{y}{b-a} \right\}^{w-1}
      \left\{ \frac{b-a-(x+y-a)}{b-a} \right\}^{n-i}
      \left( \frac{1}{b-a} \right)^{2} dx \\
 & = S_{1} y^{w-1} \left( \frac{1}{b-a} \right)^{n}
    \int_{0}^{b-y} \left\{ x-a \right\}^{i-w-1} \left\{ b-y-x \right\}^{n-i} dx
\end{align*}
Using \cite[(3.196.3)]{grad}
\begin{equation*}
\int_{\alpha}^{\beta} (x - \alpha)^{\mu - 1} (\beta - x)^{\nu - 1} dx
 = (\beta - \alpha)^{\mu + \nu - 1} B(\mu, \nu)
 = (\beta - \alpha)^{\mu + \nu - 1} ~
     \frac{(\mu - 1)! (\nu - 1)!}{(\mu + \nu - 1)!}
\end{equation*}
with $ \alpha = a $, $ \beta = b-y $, $ \mu = i-w $, $ \nu = n-i+1 $ and
$ \mu + \nu - 1 = n - w $,
\begin{align}
f_{D_{i,w,unif}}(y) \label{appeq:fdiw.unif}
 & = \frac{n!}{(i-w-1)! (w-1)! (n-i)!} ~ y^{w-1}
     \left( \frac{1}{b-a} \right)^{n}
     \left( b-y-a \right)^{n-w} \frac{(i-w-1)! (n-i)!}{(n-w)!} \nonumber \\
 & = \frac{n!}{(w-1)! (n-w)!} ~ y^{w-1} \left( \frac{1}{b-a} \right)^{n}
     \left( b-y-a \right)^{n-w}
\end{align}
If $ w = 1 $ this matches the spacing result \cite[(4)]{kreider23a}.

\subsubsection*{Expected Interval Spacing}

\begin{align*}
E\Bigl\{ D_{i,w,unif} \Bigr\}
 & = \int_{0}^{\infty} y ~ f_{D_{i,w,unif}}(y) ~ dy \\
 & = \int_{0}^{\infty} \frac{n!}{(w-1)! (n-w)!} ~ y^{w}
       \left( \frac{1}{b-a} \right)^{n} \left( b-y-a \right)^{n-w} dy \\
 & = \frac{n!}{(w-1)! (n-w)!} \left( \frac{1}{b-a} \right)^{n}
    \int_{0}^{b-a} y^{w} \left( b-a-y \right)^{n-w} dy
\end{align*}
Again using \cite[(3.196.3)]{grad} with $ \alpha = 0 $, $ \beta = b-a $,
$ \mu = w + 1 $, $ \nu = n - w + 1 $, and $ \mu + \nu - 1 = n + 1 $,
\begin{align} \label{appeq:ediw.unif}
E\Bigl\{ D_{i,w,unif} \Bigr\}
 & = \frac{n!}{(w-1)! (n-w)!} \left( \frac{1}{b-a} \right)^{n}
    \left( b - a \right)^{n+1} ~ \frac{w! (n-w)!}{(n+1)!} \nonumber \\
 & = w ~ \frac{b - a}{n + 1}
\end{align}
If $ w = 1 $ this reduces to the spacing result \cite[(5)]{kreider23a}.

\subsubsection*{Variance of Interval Spacing}

\begin{align*}
E\Bigl\{ D_{i,w,unif}^{2} \Bigr\}
 & = \int_{0}^{\infty} y^{2} ~ f_{D_{i,w,unif}}(y) ~ dy \\
 & = \int_{0}^{\infty} \frac{n!}{(w-1)! (n-w!)} ~ y^{w+1}
    \left( \frac{1}{b-a} \right)^{n} \left( b - y - a \right)^{n-w} dy \\
 & = \frac{n!}{(w-1)! (n-w)!} \left( \frac{1}{b-a} \right)^{n}
    \int_{0}^{b-a} y^{w+1} \left( b - a - y \right)^{n-w} dy
\end{align*}
Using \cite[(3.196.3)]{grad} with $ \alpha = 0 $, $ \beta = b - a $,
$ \mu = w + 2 $, $ \nu = n - w + 1 $, and $ \mu + \nu - 1 = n + 2 $,
\begin{align*}
E\Bigl\{ D_{i,w,unif}^{2} \Bigr\}
 & = \frac{n!}{(w-1)! (n-w)!} \left( \frac{1}{b-a} \right)^{n}
    \left( b - a \right)^{n+2} \frac{(w+1)! (n-w)!}{(n+2)!} \\
 & = \frac{w (w+1)}{(n+1) (n+2)} \left( b-a \right)^{2}
\end{align*}
Then
\begin{align} \label{vdiw.unif}
V\Bigl\{ D_{i,w,unif}^{2} \Bigr\}
 & = E\Bigl\{ D_{i,w}^2 \Bigr\} - E\Bigl\{ D_{i,w} \Bigr\}^2 \nonumber \\
 & = \frac{w (w+1)}{(n+1) (n+2)} \left( b-a \right)^{2} -
    \frac{w^2}{(n+1)^2} \left( b-a \right)^{2} \nonumber \\
 & = \frac{(w^{2} + w) (n+1) - w^{2} (n+2)}{(n+1)^{2} (n+2)}
    \left( b-a \right)^{2} \nonumber \\
 & = \frac{w (n+1) + w^{2} (n + 1 - (n + 2))}{n+2}
    \left( \frac{b-a}{n+1} \right)^{2} \nonumber \\
 & = \frac{w (n+1-w)}{n+2} \left( \frac{b-a}{n+1} \right)^{2}
\end{align}
With $ w = 1 $ this is the same as the spacing variance.

%%%
\subsection*{Interval Spacing for Exponential Variates}

\renewcommand{\theequation}{E.\arabic{equation}}
\setcounter{equation}{0}

The variate's density and distribution functions are
\begin{align} \label{appeq:pcdf.exp}
f_{exp}(x) & = \lambda e^{-\lambda x} \\
F_{exp}(x) & = 1 - e^{-\lambda x}
\end{align}
for $ x \ge 0 $.

\subsubsection*{Density Function}

\begin{align*}
f_{D_{i,w,exp}}(y)
 & = S_{1} 
     \begin{aligned}[t]
      \int_{-\infty}^{\infty} &
      \left\{ 1 - e^{-\lambda x} \right\}^{i-w-1}
       \left\{ \left( 1 - e^{-\lambda (x+y)} \right) -
              \left( 1 - e^{-\lambda x} \right) \right\}^{w-1}
       \left\{ 1 - \left( 1 - e^{-\lambda (x+y)} \right) \right\}^{n-i} \\
      & \cdot
       \lambda ~ e^{-\lambda x} ~ \lambda ~ e^{-\lambda (x+y)} ~ dx
     \end{aligned} \\
 & = S_{1}
    \int_{-\infty}^{\infty} \left\{ 1 - e^{-\lambda x} \right\}^{i-w-1}
      \left\{ e^{-\lambda x} - e^{-\lambda (x+y)} \right\}^{w-1}
      \left\{ e^{-\lambda (x+y)} \right\}^{n-i}
      \lambda^{2} ~ e^{-\lambda x} ~ e^{-\lambda (x+y)} ~ dx \\
 & = S_{1}
    \int_{-\infty}^{\infty} \left\{ 1 - e^{-\lambda x} \right\}^{i-w-1}
      e^{-\lambda (w-1)x} \left\{ 1 - e^{-\lambda y} \right\}^{w-1}
      ~ e^{-\lambda (n-i) x} ~ e^{-\lambda (n-i) y}
      ~ \lambda^{2} ~ e^{-2 \lambda x} ~ e^{-\lambda y} ~ dx \\
 & = S_{1}
      ~ e^{-\lambda (n-i) y} ~ e^{-\lambda y} \lambda^{2}
    \int_{-\infty}^{\infty} \left\{ 1 - e^{-\lambda x} \right\}^{i-w-1}
      e^{-\lambda (w-1) x} ~ e^{-\lambda (n-i) x} ~ e^{-2 \lambda x} ~ dx \\
 & = S_{1}
      \left\{ 1-e^{-\lambda y} \right\}^{w-1}
    \int_{0}^{\infty} \left\{ 1 - e^{-\lambda x} \right\}^{i-w-1}
      e^{-\lambda (n-i+w+1) x} dx
\end{align*}
With \cite[(3.312.1)]{grad}
\begin{equation*}
\int_{0}^{\infty} \left( 1 - e^{-x/\beta} \right)^{\nu - 1} e^{-\mu x} dx
 = \beta B(\beta \mu, \nu)
 = \beta ~ \frac{(\beta \mu - 1)! (\nu - 1)!}{(\beta \mu + \nu - 1)!}
\end{equation*}
we have $ \beta = 1/\lambda $, $ \nu = i - w $, $ \mu = (n-i+w+1) \lambda $.
Then $ \beta \mu = n - i + w + 1 $ and $ \beta \mu + \nu - 1 = n $.
Substituting,
\begin{align} \label{appeq:fdiw.exp}
f_{D_{i,w,exp}}(y)
 & = S_{1} \lambda^{2} e^{-\lambda (n-i+1) y}
      \left\{ 1-e^{-\lambda y} \right\}^{w-1}
     \frac{1}{\lambda} \frac{(n-i+w)! (i-w-1)!}{n!} \nonumber \\
 & = \frac{n!}{(i-w-1)! (w-1)! (n-i)!} \frac{(n-i+w)! (i-w-1)!}{n!}
    ~ \lambda \left\{ e^{-\lambda y} \right\}^{n-i+1}
    \left\{ 1 - e^{-\lambda y} \right\}^{w-1} \nonumber \\
 & = \frac{(n-i+w)!}{(w-1)! (n-i)!} ~ \lambda
    \left\{ e^{-\lambda y} \right\}^{n-i+1}
    \left\{ 1 - e^{-\lambda y} \right\}^{w-1}
\end{align}
Note that the pre-factor is
\begin{equation*}
 w \binom{n-i+w}{n-i}
\end{equation*}
If $ w = 1 $ this simplifies to \cite[(7)]{kreider23a}.

\subsubsection*{Expected Interval Spacing}

\begin{align*}
E\Bigl\{ D_{i,w,exp} \Bigr\}
 & = \int_{0}^{\infty} y ~ f_{D_{i,w,exp}}(y) ~ dy \\
 & = \int_{0}^{\infty} y ~ \frac{(n-i+w)!}{(w-1)! (n-i)!} ~ \lambda
    \left\{ e^{-\lambda y} \right\}^{n-i+1}
    \left\{ 1 - e^{-\lambda y} \right\}^{w-1} dy \\
 & = \frac{(n-i+w)!}{(w-1)! (n-i)!} ~ \lambda
    \int_{0}^{\infty} y \left\{ e^{-\lambda y} \right\}^{n-i+1}
    \left\{ 1 - e^{-\lambda y} \right\}^{w-1} dy
\end{align*}
Using \cite[(3.432)]{grad}
\begin{equation*}
\int_{0}^{\infty} x^{\nu - 1} e^{-\mu x} \left( e^{-x} - 1 \right)^{\alpha} dx
  = \Gamma(\nu) \sum_{k=0}^{\alpha}
   (-1)^{k} \binom{\alpha}{k} ~ \frac{1}{( \alpha + \mu - k )^{\nu}}
\end{equation*}
and making the variable change $ y = x / \lambda $, $ dy = dx / \lambda $ so
that
\begin{multline*}
\frac{(n-i+w)!}{(w-1)! (n-i)!} ~ \lambda
 \int_{0}^{\infty} \frac{x}{\lambda} \left\{ 1 - e^{-x} \right\}^{w-1}
   \left\{ e^{-x} \right\}^{n-i+1} \frac{1}{\lambda} ~ dx \\
 = \frac{(n-i+w)!}{(w-1)! (n-i)!} \frac{1}{\lambda} (-1)^{w-1}
 \int_{0}^{\infty} x \left\{ e^{-x} - 1 \right\}^{w-1}
   \left\{ e^{-x} \right\}^{n-i+1} dx
\end{multline*}
we identify $ \nu = 2 $, $ \alpha = w - 1 $, $ \mu = n - i + 1 $, and
$ \alpha + \mu = n - i + w $, giving
\begin{align} \label{appeq:ediw.exp}
E\Bigl\{ D_{i,w,exp} \Bigr\}
 = \frac{(n-i+w)!}{(w-1)! (n-i)!} \frac{1}{\lambda} (-1)^{w-1}
    \sum_{k=0}^{w-1} (-1)^{k} \binom{w-1}{k} \frac{1}{(n-i+w-k)^{2}}
\end{align}
If $ w = 1 $ the sum reduces to one term and we have $ 1 / \lambda (n-i+1) $,
which is the same as \cite[(8)]{kreider23a}.

\subsubsection*{Variance of Interval Spacing}

\begin{align*}
E\Bigl\{ D_{i,w,exp}^{2} \Bigr\}
 & = \int_{0}^{\infty} y^{2} f_{D_{i,w,exp}}(y) ~ dy \\
 & = \int_{0}^{\infty} y^{2} ~ \frac{(n-i+w)!}{(w-1)! (n-i)!} ~ \lambda
    \left\{ 1 - e^{-\lambda y} \right\}^{w-1}
    \left\{ e^{-\lambda y} \right\}^{n-i+1} dy \\
 & = \frac{(n-i+w)!}{(w-1)! (n-i)!} ~ \lambda
    \int_{0}^{\infty} \frac{1}{\lambda^{2}} ~ x^{2}
      \left\{ 1 - e^{-x} \right\}^{w-1} \left\{ e^{-x} \right\}^{n-i+1}
      \frac{1}{\lambda} ~ dx \\
 & = \frac{(n-i+w)!}{(w-1)! (n-i)!} \frac{1}{\lambda^{2}} (-1)^{w-1}
    \int_{0}^{\infty} x^{2} \left\{ e^{-x} - 1 \right\}^{w-1}
      \left\{ e^{-x} \right\}^{n-i+1} dx
\end{align*}
where we have again changed variables in the third line.  From
\cite[(3.412)]{grad} with now $ \nu = 3 $, $ \mu = n - i + 1 $,
$ \alpha = w - 1 $, $ \mu + \alpha = n - i + w $, and $ \Gamma(\nu) = 2 $,
\begin{equation} \label{appeq:ediwsq.exp}
E\Bigl\{ D_{i,w,exp}^{2} \Bigr\}
 = \frac{(n-i+w)!}{(w-1)! (n-i)!} \frac{2}{\lambda^{2}}
  \sum_{k=0}^{w-1} (-1)^{k} \binom{w-1}{k} \frac{1}{(n-i+w-k)^{3}}
\end{equation}
With the series we cannot easily square this, so the variance uses
\eqref{eq:vdiw.gen} with \eqref{appeq:ediw.exp} and it.  If $ w = 1 $
the value simplifies to $ 2 / (\lambda (n-i+1))^{2} $, which after
subtraction reduces the numerator to 1 and matches the variance of $ D_{i} $.

To evaluate this series, you must use a high precision math library.

%%%
\subsection*{Interval Spacing for Logistic Variates}

\renewcommand{\theequation}{L.\arabic{equation}}
\setcounter{equation}{0}

The variate's density and distribution functions are
\begin{align} \label{appeq:pcdf.logis.raw}
f_{logis}(x)
 & = \frac{1}{\sigma}
     \frac{e^{-(x-\mu)/\sigma}}{\left( 1 + e^{-(x-\mu)/\sigma} \right)^{2}} \\
F_{logis}(x)
 & = \frac{1}{1 + e^{-(x-\mu)/\sigma}}
\end{align}
for all x.  Substituting $ z = (x - \mu) / \sigma $ and $ dz = dx / \sigma $,
and for the shifted functions $ v = y / \sigma $
\begin{align*} \label{appeq:pcdf.logis}
f_{logis}(x)
 & \rightarrow \frac{e^{-z}}{\sigma \left( 1 + e^{-z} \right)^{2}} \\
F_{logis}(x)
 & \rightarrow \frac{1}{1 + e^{-z}} \\
f_{logis}(x+y)
 & \rightarrow \frac{e^{v} e^{-z}}{\sigma \left( e^{v} + e^{-z} \right)^{2}} \\
F_{logis}(x+y)
 & \rightarrow \frac{e^{v}}{e^{v} + e^{-z}}
\end{align*}

\subsubsection*{Density Function}

\begin{align*}
f_{D_{i,w,logis}}(y)
 & = S_{1} 
     \begin{aligned}[t]
      \int_{-\infty}^{\infty} &
       \left\{ \frac{1}{1+e^{-z}} \right\}^{i-w-1}
       \left\{ \frac{e^{v}}{e^{v}+e^{-z}} - \frac{1}{1+e^{-z}} \right\}^{w-1}
       \left\{ 1 - \frac{e^{v}}{e^{v}-e^{-z}} \right\}^{n-i} \\
      & \cdot \frac{1}{\sigma} \frac{e^{-z}}{\left( 1+e^{-z} \right)^{2}}
       \frac{1}{\sigma} \frac{e^{v} e^{-z}}{\left( e^{v}+e^{-z} \right)^{2}}
       ~ \sigma ~ dz
     \end{aligned} \\
 & = \frac{S_{1}}{\sigma}
    \begin{aligned}[t]
     \int_{-\infty}^{\infty} &
      \left\{ \frac{1}{1+e^{-z}} \right\}^{i-w-1}
      \left\{ \frac{e^{v}+e^{v}e^{-z}-e^{v}-e^{-z}}
                   {\left( e^{v}+e^{-z} \right) \left( 1+e^{-z} \right)}
              \right\}^{w-1}
      \left\{ \frac{e^{v}+e^{-z}-e^{v}}{e^{v}+e^{-z}} \right\}^{n-i} \\
     & \cdot e^{-z} \left\{ \frac{1}{1+e^{-z}} \right\}^{2}
      e^{v} e^{-z} \left\{ \frac{1}{e^{v}+e^{-z}} \right\}^{2} dz
     \end{aligned} \\
 & = \frac{S_{1}}{\sigma}
    \begin{aligned}[t]
     \int_{-\infty}^{\infty} &
      \left\{ \frac{1}{1+e^{-z}} \right\}^{i-w-1}
      \left\{ \frac{\left( e^{v}-1 \right) e^{-z}}
                   {\left( e^{v}+e^{-z} \right) \left( 1+e^{-z} \right)}
              \right\}^{w-1}
      \left\{ \frac{e^{-z}}{e^{v}+e^{-z}} \right\}^{2} \\
     & \cdot \left\{ e^{-z} \right\}^{2}
      \left\{ \frac{1}{1+e^{-z}} \right\}^{2}
      e^{v} \left\{ \frac{1}{e^{v}+e^{-z}} \right\}^{2} dz
     \end{aligned} \\
 & = \frac{S_{1}}{\sigma} ~ e^{v} \left\{ e^{v}-1 \right\}^{w-1}
    \int_{-\infty}^{\infty} \left\{ \frac{1}{1+e^{-z}} \right\}^{i-w-1+w-1+2}
      \left\{ e^{-z} \right\}^{w-1+n-i+2}
      \left\{ \frac{1}{e^{v}+e^{-z}} \right\}^{w-1+n-i+2} dz \\
 & = \frac{S_{1}}{\sigma} ~ e^{v} \left\{ e^{v}-1 \right\}^{w-1}
    \int_{-\infty}^{\infty} \left\{ \frac{1}{1+e^{-z}} \right\}^{i}
      \left\{ \frac{1}{e^{v}+e^{-z}} \right\}^{n-i+w+1}
      \left\{ e^{-z} \right\}^{n-i+w+1} dz
\end{align*}

This has the form \cite[(3.315.1)]{grad}
\begin{align*}
 \int_{-\infty}^{\infty}
   \frac{e^{-\mu x}}
        {\left( e^{\beta}+e^{-x} \right)^{\nu}
         \left( e^{\gamma}+e^{-x} \right)^{\rho}} dx
 & = e^{\gamma(\mu-\rho) - \beta\nu} B(\mu,\nu+\rho-\mu)
     ~ {}_{2}F_{1}\left(\nu, \mu; \nu+\rho; 1-e^{\gamma-\beta} \right) \\
 & = e^{\gamma(\mu-\rho) - \beta\nu} ~
     \frac{(\mu-1)! (\nu+\rho-\mu-1)!}{(\nu-\rho-1)!}
     ~ {}_{2}F_{1}\left(\nu, \mu; \nu+\rho; 1-e^{\gamma-\beta} \right)
\end{align*}
Letting $ \beta = 0 $, $ \nu = i $, $ \gamma = v $, $ \rho = n-i+w+1 $, and
$ \mu=n-i+w+1 $, this satisfies the requirements for the definite integral.
Further, $ \nu + \rho - \mu - 1 = i - 1 $, $ \nu + \rho - 1 = n + w $, and
$ \gamma (\mu - \rho) - \beta \nu = 0 $, giving
\begin{align}
f_{D_{i,w,logis}}(y)
 & = \frac{S_{1}}{\sigma} e^{v} \left\{ e^{v}-1 \right\}^{w-1} B(n-i+w+1,i)
     ~ {}_{2}F_{1}\left(i,n-i+w+1 ; n+w+1 ; 1-e^{v} \right) \nonumber \\
 & = \frac{n!}{(i-w-1)! (w-1)! (n-i)!} \frac{1}{\sigma}
     e^{v} \left\{ e^{v}-1 \right\}^{w-1}
     \frac{(n-i+w)! (i-1)!}{(n+w)!}
     ~ {}_{2}F_{1}\left(i,n-i+w+1 ; n+w+1 ; 1-e^{v} \right) \nonumber \\
 & = \frac{n!}{(n+w)!} \frac{(i-1)!}{(i-w-1)!} \frac{(n-i+w)!}{(n-i)!}
     \frac{1}{(w-1)!} \frac{1}{\sigma} e^{v} \left\{ e^{v}-1 \right\}^{w-1}
     {}_{2}F_{1}\left(i,n-i+w+1 ; n+w+1 ; 1-e^{v} \right) \nonumber \\
 & = w \left\{ \prod_{j=1}^{w} \frac{(i-j) (n-i+j)}{j (n+j)} \right\}
     \frac{1}{\sigma} e^{v} \left\{ e^{v}-1 \right\}^{w-1}
     {}_{2}F_{1}\left(i,n-i+w+1 ; n+w+1 ; 1-e^{v} \right)
\end{align}

\subsubsection*{Expected Interval Spacing}

Rather than attempting to integrate the hypergeometric function, we
swap the order of the variables to get the expected interval spacing for
the logistic function.
\begin{align*}
E\Bigl\{ D_{i,w,logis} \Bigr\}
 & = \int_{0}^{\infty} y ~ dy ~ f_{D_{i,w,logis}}(y) \\
 & = \int_{0}^{\infty} \sigma^{2} v ~ dv
     \int_{-\infty}^{\infty} \frac{S_{1}}{\sigma} e^{v}
       \left\{ e^{v}-1 \right\}^{w-1}
       \left\{ \frac{1}{e^{v}+e^{-z}} \right\}^{n-i+w+1}
       \left\{ e^{-z} \right\}^{n-i+w+1} dz \\
 & = S_{1} \sigma
    \int_{-\infty}^{\infty} dz \left\{ \frac{1}{1+e^{-z}} \right\}^{i}
      \left\{ e^{-z} \right\}^{n-i+w+1}
    \int_{0}^{\infty} v e^{v} \left\{ e^{v}-1 \right\}^{w-1}
      \left\{ \frac{1}{e^{v}+e^{-z}} \right\}^{n-i+w+1} dv \\
 & = S_{1} \sigma
    \int_{-\infty}^{\infty} dz \left\{ \frac{1}{1+e^{-z}} \right\}^{i}
      \left\{ e^{-z} \right\}^{n-i+w+1} I_{in}
\end{align*}

To evaluate the inner integral, we will first evaluate by parts which will
give a series, and then will expand a polynomial in a second series.  First
we will need a series solution to an indefinite integral.  From
\cite[(2.153)]{grad}
\begin{equation*}
 \int \frac{(c + xd)^{\nu}}{(a + xb)^{\mu}} ~ dx
  = \frac{1}{-(\mu-\nu-1)} \frac{1}{b} \frac{(c+dx)^{\nu}}{(a+xb)^{\mu-1}}
   - \frac{1}{-(\mu-\nu-1)} \frac{ad-bc}{b}
      \int \frac{(c+xd)^{\nu-1}}{(a+xb)^{\mu}} ~ dx
\end{equation*}
In general, one step is
\begin{align*}
\int \frac{(c+xd)^{\nu-k}}{(a+xb)^{\mu}} ~ dx
 & = \frac{1}{-(\mu-\nu+k-1)} \frac{1}{b} \frac{(c+xd)^{\nu-k}}{(a+xb)^{\mu-1}}
    - \frac{1}{-(\mu-\nu+k-1)} \frac{ad-bc}{b}
      \int \frac{(c+xd)^{\nu-(k+1)}}{(a+xb)^{\mu}} ~ dx \\
 & = -A_{k} + B_{k} \int \frac{(c+xd)^{\nu-(k+1)}}{(a+xb)^{\mu}} ~ dx
\end{align*}
The recursion down the chain follows
\begin{align*}
\int \frac{(c+xd)^{\nu-k}}{(a+xb)^{\mu}} dx
 & = -A_{0} + B_{0} \int \frac{(c+xd)^{\nu-1}}{(a+xb)^{\mu}} ~ dx \\
 & = -A_{0} +
    B_{0} \left[
      -A_{1} + B_{1} \int \frac{(c+xd)^{\nu-2}}{(a+xb)^{\mu}} ~ dx \right] \\
 & = -A_{0} - A_{1} B_{0} +
    B_{0} B_{1} \left[
      -A_{2} + B_{2} \int \frac{(c+xd)^{\nu-3}}{(a+xb)^{\mu}} ~ dx \right] \\
 & = -A_{0} - A_{1} B_{0} - A_{2} B_{0} B_{1} +
    B_{0} B_{1} B_{2} \left[
      -A_{3} + B_{3} \int \frac{(c+xd)^{\nu-4}}{(a+xb)^{\mu}} ~ dx \right]
\end{align*}
so at the last step, with $ k = \nu $,
\begin{equation*}
\int \frac{(c+xd)^{\nu-k}}{(a+xb)^{\mu}} ~ dx
 = -A_{0} - \sum_{k=1}^{\nu-1} A_{k} \prod_{l=0}^{k-1} B_{l}
   + \left\{ \prod_{l=0}^{\nu-1} B_{l} \right\} \int \frac{dx}{(a+xb)^{\mu}}
\end{equation*}
This termination is, via \cite[(2.111.1)]{grad}
\begin{equation*}
\int (a+xb)^{\rho} ~ dx = \frac{1}{b (\rho+1)} ~ (a+xb)^{\rho+1}
\end{equation*}
with $ \rho = -\mu $.  This gives
\begin{align*}
\int \frac{dx}{(a+xb)^{\mu}}
 & = \frac{1}{b(-\mu + 1)} ~ (a+xb)^{-\mu+1} \\
 & = \frac{1}{b(-\mu + 1)} \frac{1}{(a+bx)^{\mu-1}} \\
 & = -A_{\nu}
\end{align*}
The recursion chain is now
\begin{align*}
\int \frac{(c+xd)^{\nu}}{(a+xb)^{\mu}} dx
 & = -A_{0} - \sum_{k=1}^{\nu-1} A_{k} \prod_{l=0}^{k-1} B_{l}
     -A_{\nu} \prod_{l=0}^{\nu-1} B_{l} \\
 & = -A_{0} - \sum_{k=1}^{\nu} A_{k} \prod_{l=0}^{k-1} B_{l}
\end{align*}

The product simplifies
\begin{align*}
\prod_{l=0}^{k-1} B_{l}
 & = \prod_{l=0}^{k-1} \frac{\nu-l}{\mu-\nu+l-1} \frac{ad-bc}{b} \\
 & = \left( \frac{ad-bc}{b} \right)^{k}
    \frac{\nu (\nu-1) (\nu-2) \ldots (\nu-k+1)}
         {(\mu-\nu-1) (\mu-\nu) (\mu-\nu+1) \ldots (\mu-\nu+k-2)} \\
 & = \left( \frac{ad-bc}{b} \right)^{k} \frac{\nu!}{(\nu-k)!}
     \frac{\mu-\nu-2)!}{(\mu-\nu+k-2)!}
\end{align*}
Substituting this back in,
\begin{align*}
\int \frac{(c+xd)^{\nu}}{(a+xb)^{\mu}} ~ dx
 & = -A_{0} -
     \sum_{k=1}^{\nu} A_{k} \left( \frac{ad-bc}{b} \right)^{k}
       \frac{\nu!}{(\nu-k)!} \frac{\mu-\nu-2)!}{(\mu-\nu+k-2)!} \\
 & = -A_{0} -
     \sum_{k=1}^{\nu} \frac{1}{\mu-\nu+k-1} \frac{1}{b}
       \frac{(c+xd)^{\nu-k}}{(a+xb)^{\mu-1}} \left( \frac{ad-bc}{b} \right)^{k}
       \frac{\nu!}{(\nu-k)!} \frac{\mu-\nu-2)!}{(\mu-\nu+k-2)!} \\
 & = -A_{0} -
     \frac{\nu! (\mu-\nu-2)!}{b (a+xb)^{\mu-1}}
     \sum_{k=1}^{\nu} (c+xd)^{\nu-k} \left( \frac{ad-bc}{b} \right)^{k}
       \frac{1}{(\nu-k)!} \frac{1}{(\mu-\nu+k-1)!}
\end{align*}
At $ k = 0 $ the second term simplies to $ A_{0} $ and we can fold it into
the series.  The final, general solution of this indefinite integral is
\begin{equation} \label{eq:2.153}
\int \frac{(c+xd)^{\nu}}{(a+xb)^{\mu}} ~ dx
 = - \frac{\nu! (\mu-\nu-2)!}{b (a+bx)^{\mu-1}}
    \sum_{k=0}^{\nu} (c+xd)^{\nu-k} \left( \frac{ad-bc}{b} \right)^{k}
      \frac{1}{(\nu-k)!} \frac{1}{(\mu-\nu+k-1)!}
\end{equation}

To solve $ I_{in} $ we work by parts, which will require \eqref{eq:2.153}.
Let $ t = v $, $ dt = dv $, and
\begin{align*}
 du & = e^{v} \left\{ e^{v}-1 \right\}^{w-1}
        \left\{ \frac{1}{e^{v}+e^{-z}} \right\}^{n-i+w-1} \\
    & = \left\{ r-1 \right\}^{w-1} \left\{ \frac{1}{r+e^{-z}} \right\}^{n-i+w+1}
\end{align*}
making the further substitution $ r = e^{v} $ and $ dr = e^{v} dv $.  This is
in the form of \eqref{eq:2.153} with $ a = e^{-z} $, $ b = 1 $, $ c = -1 $,
$ d = 1 $, $ \nu = w-1 $, $ \mu = n-i+w+1 $, and $ \nu - \mu - 1 = n-i+1 $.
So
\begin{align*}
 u & = - (w-1)! (n-i)! \left\{ \frac{1}{e^{v}+e^{-z}} \right\}^{n-i+w}
      \sum_{k=0}^{w-1} \frac{1}{(w-1-k)!} \frac{1}{(n-i+1+k)!}
        \left\{ \frac{ e^{-z}+1 }{1} \right\}^{k}
        \left\{ e^{v}-1 \right\}^{w-1-k} \\
   & = - (w-1)! (n-i)! \left\{ \frac{1}{e^{v}+e^{-z}} \right\}^{n-i+w}
      \sum_{k=0}^{w-1} \frac{1}{(w-1-k)!} \frac{1}{(n-i+1+k)!}
        \left\{ 1+e^{-z} \right\}^{k} \left\{ e^{v}-1 \right\}^{w-1-k}
\end{align*}
Then
\begin{align*}
I_{in}
 & = \int_{0}^{\infty} v ~ e^{v} \left\{ e^{v}-1 \right\}^{w-1}
       \left\{ \frac{1}{e^{v}+e^{-z}} \right\}^{n-i+w+1} dv \\
 & = \left[ tu \right]_{0}^{\infty} - \int_{0}^{\infty} u ~ dt \\ 
 & = \left[ - (w-1)! (n-i)! \left\{ \frac{1}{e^{v}+e^{-z}} \right\}^{n-i+w} v
        \sum_{k=0}^{w-1} \frac{1}{(w-1-k)!} \frac{1}{(n-i+1+k)!} 
          \left\{ 1+e^{-z} \right\}^{k} \left\{ e^{v}-1 \right\}^{w-1-k}
     \right]_{0}^{\infty} \\
  & \qquad + \int_{0}^{\infty} (w-1)! (n-i)!
       \left\{ \frac{1}{e^{v}+e^{-z}} \right\}^{n-i+w}
        \sum_{k=0}^{w-1} \frac{1}{(w-1-k)!} \frac{1}{(n-i+1+k)!}
          \left\{ 1+e^{-z} \right\}^{k} \left\{ e^{v}-1 \right\}^{w-1-k} \\
 & = \int_{0}^{\infty} (w-1)! (n-i)!
    \sum_{k=0}^{w-1} \frac{1}{(w-1-k)!} \frac{1}{(n-i+1+k)!}
          \left\{ 1+e^{-z} \right\}^{k} \left\{ e^{v}-1 \right\}^{w-1-k}
          \left\{ \frac{1}{e^{v}+e^{-z}} \right\}^{n-i+w} dv \\
 & = \sum_{k=0}^{w-1} \frac{(w-1)!}{(w-1-k)!} \frac{(n-i)!}{(n-i+1+k)!}
    \left\{ 1+e^{-z} \right\}^{k} \int_{0}^{\infty} \left\{ e^{v}-1 \right\}^{w-1-k}
    \left\{ \frac{1}{e^{v}+e^{-z}} \right\}^{n-i+w} dv
\end{align*}
The square brackets in the third step goes to zero at both bounds, with 
$ 1/e^{v} $ dominating at infinity and $ v $ at 0.

To evaluate this integral we now expand the first factor as a polynomial
using \cite[(1.111)]{grad}
\begin{align*}
(a + x)^{\nu}
 & = \sum_{l=0}^{\nu} \binom{\nu}{l} x^{l} a^{\nu-l} \\
 & = a^{\nu} + \nu a^{\nu-1} x + \sum_{l=2}^{\nu} \binom{\nu}{l} a^{\nu-l} x^{l}
\end{align*}
The first two terms have been expanded from the series because they will
integrate simply.  We have $ \nu = w-1-k $ and $ a = -1 $ for $ x = e^{v} $.
The second term will disappear if $ \nu = 0 $ or $ k = w-1 $.  Ignore the
sum if $ \nu < 2 $, which occurs at $ w = 2 $ or $ k > w-2 $.  So
\begin{align*}
\int_{0}^{\infty} & \left\{ e^{v}-1 \right\}^{w-1-k} \left\{ \frac{1}{e^{v}+e^{-z}} \right\}^{n-i+w} dv \\
 & = \int_{0}^{\infty} (-1)^{w-1-k} \left\{ \frac{1}{e^{v}+e^{-z}} \right\}^{n-i+w} dv \\
 & \qquad + \int_{0}^{\infty} (w-1-k) (-1)^{w-2-k} e^{v}
        \left\{ \frac{1}{e^{v}+e^{-z}} \right\}^{n-i+w} dv \\
 & \qquad + \sum_{l=2}^{w-1-k} \binom{w-1-k}{l} (-1)^{w-1-k}
        \int_{0}^{\infty} \left\{ e^{v} \right\}^{l}
                          \left\{ \frac{1}{e^{v}+e^{-z}} \right\}^{n-i+w} dv
\end{align*}

For the first integral we substitute $ r = e^{v}+e^{-z} $,
$ dr = e^{v} dv = (r - e^{-z}) dv $.  We will also need \cite[(2.117.4)]{grad}
\begin{align*}
\int \frac{dx}{x^{\nu} (a+xb)}
 & = \frac{(-1)^{\nu} b^{\nu-1}}{a^{\nu}} ~ \ln \frac{a+xb}{x}
    + \sum_{l=1}^{\nu-1} \frac{(-1)^{l} b^{l-1}}{(\nu-l)} a^{l}
                         \frac{1}{x^{\nu-l}} \\
 & = \frac{1}{b} \left( -\frac{b}{a} \right)^{\nu} \ln \frac{a+xb}{x}
    + \sum_{l=1}^{\nu-1} \frac{1}{\nu-l} \frac{1}{b}
          \left( -\frac{b}{a} \right)^{l} \left( \frac{1}{x} \right)^{\nu-l}
\end{align*}
letting $ \nu = n-i+w $, $ a = -e^{-z} $, and $ b = 1 $.
\begin{align*}
\int_{0}^{\infty} & \left\{ \frac{1}{e^{v}+e^{-z}} \right\}^{n-i+w} dv \\
 & = \int \left\{ \frac{1}{r} \right\}^{n-i+w} \left\{ \frac{1}{r-e^{-z}} \right\} dr \\
 & = \left\{ \frac{1}{e^{-z}} \right\}^{n-i+w} \ln \frac{r-e^{-z}}{r}
    + \sum_{l=1}^{n-i+w-1} \frac{1}{n-i+w-l} \left\{ \frac{1}{e^{-z}} \right\}^{l}
       \left\{ \frac{1}{r} \right\}^{n-i+w-l} \\
 & = \left[ \left\{ \frac{1}{e^{-z}} \right\}^{n-i+w} \ln \frac{e^{v}}{e^{v}+e^{-z}}
    + \sum_{l=1}^{n-i+w-1} \frac{1}{n-i+w-l} \left\{ \frac{1}{e^{-z}} \right\}^{l}
       \left\{ \frac{1}{e^{v}+e^{-z}} \right\}^{n-i+w-l} \right]_{0}^{\infty} \\
 & = \left\{ \frac{1}{e^{-z}} \right\}^{n-i+w} \ln \left\{ 1+e^{-z} \right\}
    + \sum_{l=1}^{n-i+w-1} \frac{1}{n-i+w-l} \left\{ \frac{1}{e^{-z}} \right\}^{l}
       \left\{ \frac{1}{1+e^{-z}} \right\}^{n-i+w-l} 
\end{align*}
At $ v = \infty $ both terms go to 0, and at the lower bound $ e^{v} $ is 1.

For the second integral we substitute $ r = e^{v} $, $ dr = e^{v} dv $, and
use \cite[(2.111.1)]{grad}
\begin{equation*}
\int (a+xb)^{\mu} dx = \frac{1}{b (\mu+1)} ~ (a + xb)^{\mu + 1}
\end{equation*}
letting $ \mu = -(n-i+w) $, $ a = e^{-z} $, and $ b = 1 $.
\begin{align*}
\int_{0}^{\infty} e^{v} \left\{ \frac{1}{e^{v}+e^{-z}} \right\}^{n-i+w} dv
 & = \int \left\{ \frac{1}{r+e^{-z}} \right\}^{n-i+w} dr \\
 & = \left[ \frac{1}{-(n-i+w+1)} \left\{ \frac{1}{e^{v}+e^{-z}} \right\}^{n-i+w-1}
     \right]_{0}^{\infty} \\
 & = \frac{1}{n-i+w-1} \left\{ \frac{1}{1+e^{-z}} \right\}^{n-i+w-1}
\end{align*}
where the integral is zero at the upper bound and again $ e^{v} \rightarrow 1 $
at the lower.

After making the same $ r $ substitution, the third integral takes the form
of \eqref{eq:2.153} with $ a = e^{-z} $, $ b = 1 $, $ c = 0 $, $ d = 1 $,\
$ \mu = n-i+w $, $ \nu = l - 1 $, and $ \mu - \nu -1 = n - i + w - l $.
\begin{align*}
\int_{0}^{\infty} &
 \left\{ e^{v} \right\}^{l-1} \left\{ \frac{1}{e^{v}+e^{-z}} \right\}^{n-i+w}
 e^{v} ~ dv \\
  & = \int r^{l-1} \left\{ \frac{1}{r+e^{-z}} \right\}^{n-i+w} dr \\
  & = \left[ - (l-1)! (n-i+w-l-1)! \left\{ \frac{1}{e^{v}+e^{-z}} \right\}^{n-i+w-1}
     \sum_{j=0}^{l-1} \frac{1}{(l-1-j)!} \frac{1}{(n-i+w-l+j)!} \left\{ e^{-z} \right\}^{j}
       \left\{ e^{v} \right\}^{l-1-j} \right]_{0}^{\infty} \\
  & = (l-1)! (n-i+w2-l-1)! \left\{ \frac{1}{1+e^{-z}} \right\}^{n-i+w-1}
     \sum_{j=0}^{l-1} \frac{1}{(l-1-j)!} \frac{1}{(n-i+w-l+j)!} \left\{ e^{-z} \right\}^{j}
\end{align*}
with the same behavior at the upper and lower bounds.

Assembling the three integrals, we get
\begin{align}
I_{in}
 & = \int_{0}^{\infty} v e^{v} \left\{ e^{v}-1 \right\}^{w-1}
        \left\{ \frac{1}{e^{v}+e^{-z}} \right\}^{n-i+w+1} dv \nonumber \\
 & = \sum_{k=0}^{w-1} S_{3}
       \left\{ 1+e^{-z} \right\}^{k} \int_{0}^{\infty} \left\{ e^{v}-1 \right\}^{w-1-k}
         \left\{ \frac{1}{e^{v}+e^{-z}} \right\}^{n-i+w} dv \nonumber \\
 & = \sum_{k=0}^{w-1} S_{3}
    \left\{ 1+e^{-z} \right\}^{k}
    \left[
    \begin{aligned}
      (-1)^{w-1-k} \int_{0}^{\infty} \left\{ \frac{1}{e^{v}+e^{-z}} \right\}^{n-i+w} dv \\
     + (w-1-k) (-1)^{w-2-k} \int_{0}^{\infty} e^{v}
       \left\{ \frac{1}{e^{v}+e^{-z}} \right\}^{n-i+w} dv \\
     + \sum_{l=2}^{w-1-k} \binom{w-1-k}{l} (-1)^{w-1-k-l}
         \int_{0}^{\infty} \left\{ e^{v} \right\}^{l}
            \left\{ \frac{1}{e^{v}+e^{-z}} \right\}^{n-i+w} dv
    \end{aligned}
    \right] \nonumber \\
 & = \sum_{k=0}^{w-1} S_{3}
    (-1)^{w-1-k} \left\{ 1+e^{-z} \right\}^{k}
    \left[
    \begin{aligned}
      \left\{ \frac{1}{e^{-z}} \right\}^{n-i+w} \ln \left\{ 1+e^{-z} \right\} \\
     - \left\{ \sum_{l=1}^{n-i+w-1} \frac{1}{n-i+w-1} \left\{ \frac{1}{e^{-z}} \right\}^{l}
         \left\{ \frac{1}{1+e^{-z}}^{n-i+w-l} \right\}
       \right\} \\
     - \frac{w-1-k}{n-i+w-1} \left\{ \frac{1}{1+e^{-z}} \right\}^{n-i+w-1} \\
     + \left\{
       \begin{aligned}
        \sum_{l=2}^{w-1-k} \binom{w-1-k}{l} (-1)^{l} (l-1)! (n-i+w-l-1)!
          \left\{ \frac{1}{1+e^{-z}} \right\}^{n-i+w-1} \\
          \cdot \sum_{j=0}^{l-1} \frac{1}{(l-1-j)!} \frac{1}{(n-i+w-l-j)!}
           \left\{ e^{-z} \right\}^{j}
       \end{aligned} \right\}
    \end{aligned}
    \right] \nonumber \\
 & = \sum_{k=0}^{w-1} S_{3}
    (-1)^{w-1-k}
    \left[
    \begin{aligned}
      \left\{ 1+e^{-z} \right\}^{k} \left\{ \frac{1}{e^{-z}} \right\}^{n-i+w} \ln \left\{ 1+e^{-z} \right\} \\
    - \left\{ \sum_{l=1}^{n-i+w-1} \frac{1}{n-i+w-l} \left\{ \frac{1}{e^{-z}} \right\}^{l}
           \left\{ \frac{1}{1+e^{-z}} \right\}^{n-i+w-k-l}
      \right\} \\
    - \frac{w-1-k}{n-i+w-1} \left\{ \frac{1}{1+e^{-z}} \right\}^{n-i+w-k-1} \\
    + \sum_{l=2}^{w-1-k} \binom{w-1-k}{l} (-1)^{l}
        \sum_{j=0}^{l-1} \frac{(l-1)!}{(l-1-j)!}
          \frac{(n-i+w-l-1)!}{(n-i+w-l+j)!}
          \left\{ \frac{1}{1+e^{-z}} \right\}^{n-i+w-1-k}
          \left\{ e^{-z} \right\}^{l}
    \end{aligned}
    \right] \\
S_{3} & = \frac{(w-1)!}{(w-1-k)!} \frac{(n-i)!}{(n-i+1+k)!} \nonumber
\end{align}          

We can simplify the scaling factors in the last term, canceling the $ (l-1)! $
from the binomial coefficient and leaving a factor of $ 1/l $.  For
calculations the fractions of similar factorials reduce further to products.
\begin{align*}
\binom{w-1-k}{l} & \frac{(l-1)!}{(l-1-j)!} \frac{(n-i+w-1-l)!}{(n-i+w-l+j)!} \\
 & = \frac{(w-1-k)!}{l! (w-1-k-l)!} \frac{(l-1)!}{(l-1-j)!}
    \frac{(n-i+w-l-1)!}{(n-i+w-l+j)!} \\
 & = \frac{1}{l} \frac{1}{(l-1-j)!} \frac{(w-1-k)!}{(w-1-k-l)!}
    \frac{(n-i+w-l-1)!}{(n-i+w-l+j)!} \\
 & = \frac{1}{l} \frac{1}{(l-1-j)!}
     \left[ \prod_{p=0}^{l-1} w-1-k-p \right]
     \left[ \prod_{p=0}^{j} \frac{1}{n-i+w-j+p} \right]
\end{align*}

The expected interval spacing is now, with the inner integral known,
\begin{align*}
E\Bigl\{ D_{i,w,logis} \Bigr\}
 & = S_{1} \sigma \int_{-\infty}^{\infty} dz
      \left\{ \frac{1}{1+e^{-z}} \right\}^{i}
      \left\{ e^{-z} \right\}^{n-i+w+1} I_{in} \\
% & = \frac{n!}{(i-w-1)! (w-1)! (n-i)!} \sigma
 & = S_{1} \sigma
   \int_{-\infty}^{\infty}
     dz \left\{ \frac{1}{1+e^{-z}} \right\}^{i}
     \left\{ e^{-z} \right\}^{n-i+w+1}
   \sum_{k=0}^{w-1} \frac{(w-1)!}{(w-1-k)!} \frac{(n-i)!}{(n-i+1+k)!} \\
 & \quad \cdot \left[
    \begin{aligned}
      \left\{ \frac{1}{1+e^{-z}} \right\}^{-k} \left\{ e^{-z} \right\}^{-n+i-w} \ln \left\{ 1+e^{-z} \right\} \\
      - \left\{ \sum_{l=1}^{n-i+w-1} \frac{1}{n-i+w-l}
             \left\{ \frac{1}{1+e^{-z}} \right\}^{n-i+w-k-l} \left\{ e^{-z} \right\}^{-l} \right\} \\
      - \frac{w-1-k}{n-i+w-1} \left\{ \frac{1}{1+e^{-z}} \right\}^{n-i+w-k-1} \\
      + \sum_{l=2}^{w-1-k} (-1)^{l}
         \sum_{j=0}^{l-1} \frac{1}{l} \frac{1}{(l-1-j)!}
           \frac{(w-1-k)!}{(w-1-k-l)!} \frac{(n-i+w-l-1)!}{(-i+w-l+j)!}
           \left\{ \frac{1}{1+e^{-z}} \right\}^{n-i+w-1-k} \left\{ e^{-z} \right\}^{-j}
    \end{aligned}
    \right] \\
 & = \sum_{k=0}^{w-1} \frac{n!}{(i-w-1)! (w-1-k)! (n-i+1+k)!} \sigma
      (-1)^{w-1-k} \\
 & \quad \cdot \left[
    \begin{aligned}
      \int_{-\infty}^{\infty} & dz \left\{ \frac{1}{1+e^{-z}}
        \right\}^{i-k} \left\{ e^{-z} \right\}^{i} \ln \left\{ 1+e^{-z} \right\} \\
      - \sum_{l=1}^{n-i+w-1} \frac{1}{n-i+w-l}
        \int_{-\infty}^{\infty} & dz \left\{ \frac{1}{1+e^{-z}} \right\}^{n+w-k-l}
          \left\{ e^{-z} \right\}^{n-i+w+1-l} \\
      - \frac{w-1-k}{n-i+w-1} \int_{-\infty}^{\infty} &
         dz \left\{ \frac{1}{1+e^{-z}} \right\}^{n+w-k-1} \left\{ e^{-z} \right\}^{n-i+w+1} \\
      + \sum_{l=2}^{w-1-k} (-1)^{l} \sum_{j=0}^{l-1} &
          \frac{1}{l} \frac{1}{(l-1-j)!} \frac{(w-1-k)!}{(w-1-k-l)!}
          \frac{(n-i+w-l-1)!}{(n-i+w-l+j)!} \\
        & \quad \cdot
          \int_{-\infty}^{\infty} dz \left\{ \frac{1}{1+e^{-z}} \right\}^{n+w-1-k}
            \left\{ e^{-z} \right\}^{n-i+w+1+j}
    \end{aligned}
    \right]
\end{align*}

There are four integrals in the last lines, but only two unique forms.
For the first term we will use \cite[(4.293.14)]{grad}
\begin{equation*}
\int_{0}^{\infty} \frac{x^{\nu-1}}{(\gamma + x)^{\mu}} ~ \ln(\gamma + x) ~ dx
 = \gamma^{\nu-\mu} B(\nu, \mu-\nu)
   \left[ \psi(\mu) - \psi(\mu-\nu) + \ln \gamma \right]
\end{equation*}
along with $ \nu = 1 $, $ \mu = i-k $, $ \mu-\nu = i-k-1 $.  The conditions
on the integral, $ \mu > \nu > 0 $ hold at all $ k $, since $ i > w $.  The
first term becomes
\begin{align*}
\int_{-\infty}^{\infty} dz \left\{ \frac{1}{1+e^{-z}} \right\}^{i-k} e^{-z}
 \ln \left\{ 1 + e^{-z} \right\}
 & = 1^{k+1-i} B(1, i-k-1) \left[ \psi(i-k) - \psi(i-k-1) + \ln 1 \right] \\
 & = B(1, i-k-1) \left[ \psi(i-k) - \psi(i-k-1) \right] \\
 & = \frac{1}{i-k-1} \left[ \psi(i-k) - \psi(i-k-1) \right]
\end{align*}

The other three integrals fit \cite[(8.380.3)]{grad}
\begin{equation*}
\int_{0}^{\infty} \frac{t^{x-1}}{(1+t)^{x+y}} ~ dx
 = B(x,y) = \frac{(x-1)! (y-1)!}{(x+y-1)!}
\end{equation*}
This would also follow from \eqref{eq:2.153}, because at the upper bound
the terms are zero and at the lower bound only the lead, non-series term
survives.  This is equivalent to the beta function.  We make the substitution
$ r = e^{-z} $, $ dr = -e^{-z} dz $ to transform
\begin{align*}
\int_{-\infty}^{\infty} dz \left\{ \frac{1}{1+e^{-z}} \right\}^{\mu}
 \left\{ e^{-z} \right\}^{\nu}
 & = \int_{\infty}^{0} - dr \left\{ \frac{1}{1+r} \right\}^{\mu} r^{\nu-1} \\
 & = \int_{0}^{\infty} dr \left\{ \frac{1}{1+r} \right\}^{\mu} r^{\nu-1} \\
 & = B(\nu, \mu-\nu) \\
 & = \frac{(\nu-1)! (\mu-\nu-1)!}{(\mu-1)!}
\end{align*}
having let $ x = \nu $ and $ y = \mu - \nu $ for the known integral.  We have
for the
\begin{center}
\begin{tabular}{llll}
second term & $ \nu = n-i+w+1-l $ & $ \mu = n+w-k-l $ & $\mu-\nu = i-k-1 $ \\
third term  & $ \nu = n-i+w+1$    & $ \mu = n+w-1-k $ & $\mu-\nu = i-k-2 $ \\
fourth term & $ \nu = n-i+w+1+j $ & $ \mu = n+w-1-k $ & $\mu-\nu = i-k-2-j $
\end{tabular}
\end{center}

The final solution for the expected interval spacing is
\begin{align}
E\Bigl\{ D_{i,w,logis} \Bigr\}
 = \sum_{k=0}^{w-1} &
   \frac{n!}{(i-w-1)! (w-1-k)! (n-i+1+k)!} \sigma (-1)^{w-1-k} \nonumber \\
 & \cdot \left[
   \begin{aligned}
   \frac{1}{i-k-1} \left[ \psi(i-k) - \psi(i-k-1) \right] \\
   - \sum_{l=1}^{n-i+w-1} \frac{1}{n-i+w-l} ~ B(n-i+w+1-l, i-k-1) \\
   - \frac{w-1-k}{n-i+w-1} ~ B(n-i+w+1, i-k-2) \\
   + \sum_{l=2}^{w-1-k} (-1)^{l}
      \sum_{j=0}^{l-1} 
       \frac{(w-1-k)!}{(w-1-k-l)!} \frac{(n-i+w-l-1)!}{(n-i+w-l+j)!}
       \frac{B(n-i+w+1+j, i-k-2-j)}{l (l-1-j)!}
   \end{aligned} \right]
\end{align}

\bibliographystyle{amsplain}
\bibliography{dmodal}

\end{document}
